# Supplementary material for: Zero-information limit of a collective olfactory search model
Source: arXiv:2601.22233 ancillary file (2026-01-29)
Supplement: Supplementary file 1 [file SM_Zero-information_limit_of_a_collective_olfactory_search_model.pdf]

# Zero-information limit of a collective olfactory search model
# Supplementary Material

Francesco Boccardo,[1] Simone Di Marino,[2] and Agnese Seminara[1]

[1]*MaLGa, Department of Civil, Chemical and Environmental Engineering, University of Genoa, Genoa, Italy*
[2]*MaLGa, Department of Mathematics, University of Genoa, Genoa, Italy*

(Dated: January 29, 2026)

## I. CODE AVAILABILITY

All the code required to generate the results presented in this work is publicly available at `https://github.com/PimLb/olfactory-search-model`. The repository includes detailed instructions on how to run the simulations and reproduce the figures.

## II. ANALYTICAL RESULTS

We look at possible analytical prediction of the system in the two different asymptotic regimes $\beta \to 0$ and $\beta \to 1$. We analyze both of these regimes only in the infinite visual range: while it would be interesting to generalize to finite visual radius, we expect that the role of the trust parameter is better highlighted in the infinite radius regime since every agent is influenced by any other agent. A key quantity in this case will be $\boldsymbol{v}_{\text{cm}}$, the velocity of the center of mass. In fact

$$\boldsymbol{v}_i^{\text{pub}}(t) = v_0 \frac{\sum_{j\sim i} v_j(t-t_{\text{mem}})}{\|\sum_{j\sim i} v_j(t-t_{\text{mem}})\|} = v_0 \frac{\boldsymbol{v}_{\text{cm}}(t-t_{\text{mem}})}{\|\boldsymbol{v}_{\text{cm}}(t-t_{\text{mem}})\|} + O\Big(\frac{v_0}{\|\boldsymbol{v}_{\text{cm}}(t-t_{\text{mem}})\| N}\Big).$$

In particular, as long as $v_0/N \ll \|\boldsymbol{v}_{\text{cm}}\|$, we can assume that $\boldsymbol{v}_i^{\text{pub}}$ does not depend on $i$. From now on our standing assumption in this section will therefore be

$$\boldsymbol{v}_i^{\text{pub}}(t) = \boldsymbol{v}^{\text{pub}}(t) = v_0 \frac{\boldsymbol{v}_{\text{cm}}(t-t_{\text{mem}})}{\|\boldsymbol{v}_{\text{cm}}(t-t_{\text{mem}})\|}. \tag{1}$$

### A. Very high trust parameter: Langevin dynamics

We observe that with a high trust parameter we expect the agent to align their behavior immediately, with their private velocity being just a perturbation of the public one. Recall that $\boldsymbol{v}_i(t) = v_0 \frac{(1-\beta)\boldsymbol{v}_i^{\text{priv}}(t)+\beta \boldsymbol{v}^{\text{pub}}(t)}{\|(1-\beta)\boldsymbol{v}_i^{\text{priv}}(t)+\beta \boldsymbol{v}^{\text{pub}}(t)\|}$. Since here we are assuming $\beta \sim 1$, we can expand the nonlinearity using that $\|\boldsymbol{v}^{\text{pub}}\| = v_0$ and obtain that up to $O((1-\beta)^2)$ we have

$$\boldsymbol{v}_i(t) = \boldsymbol{v}^{\text{pub}}(t) + (1-\beta) P_{\boldsymbol{v}^{\text{pub}}(t)^\perp}(\boldsymbol{v}_i^{\text{priv}}(t)). \tag{2}$$

Here we denoted by $P_v : \mathbb{R}^2 \to \mathbb{R}^2$ the linear projection operator on the linear space generated by $v$, that is $P_v(w) = \frac{\langle v,w\rangle}{\|v\|^2} v$. Taking the average we obtain

$$\boldsymbol{v}_{\text{cm}}(t) = \langle \boldsymbol{v}_i(t)\rangle = \boldsymbol{v}^{\text{pub}}(t) + (1-\beta) P_{\boldsymbol{v}^{\text{pub}}(t)^\perp}(\langle \boldsymbol{v}_i^{\text{priv}}(t)\rangle). \tag{3}$$

In particular $\|\boldsymbol{v}_{\text{cm}}(t)\| \approx v_0$ with an error $O((1-\beta)^2)$: we can substitute this estimate in Equation (1) to get $\boldsymbol{v}^{\text{pub}}(t) = \boldsymbol{v}_{\text{cm}}(t-t_{\text{mem}})$; in the end we get an evolution equation for $\boldsymbol{v}_{\text{cm}}$ alone

$$\boldsymbol{v}_{\text{cm}}(t) = \boldsymbol{v}_{\text{cm}}(t-t_{\text{mem}}) + (1-\beta) P_{\boldsymbol{v}_{\text{cm}}(t-t_{\text{mem}})^\perp}(\langle \boldsymbol{v}_i^{\text{priv}}(t)\rangle).$$

This can be seen as a discretization of the following ODE:

$$\dot{\boldsymbol{v}}_{cm}(t) = \frac{1-\beta}{t_{\text{mem}}} P_{\boldsymbol{v}_{\text{cm}}(t)^\perp}(\langle \boldsymbol{v}_i^{\text{priv}}(t)\rangle). \tag{4}$$

In particular, given the same initial conditions and the scheduling for $\boldsymbol{v}_i^{\text{priv}}$, the equation is dependent only on the parameter $\frac{1-\beta}{t_{\text{mem}}}$, which dictates how fast the velocity $\boldsymbol{v}_{\text{cm}}$ is aligning to $\langle \boldsymbol{v}_i^{\text{priv}}(t)\rangle$. In order to get a clearer picture we consider the angles $\theta(t)$ and $\theta_w(t)$ that $\boldsymbol{v}_{\text{cm}}$ and $\langle \boldsymbol{v}_i^{\text{priv}}(t)\rangle$ respectively make with the $x$-axis. Letting then $w(t) = \|\langle \boldsymbol{v}_i^{\text{priv}}(t)\rangle\|$ the ODE in (4) reads as

$$\dot{\theta}(t) = \frac{(1-\beta)w(t)}{t_{\text{mem}}} \cdot \sin(\theta_w(t) - \theta(t)). \tag{5}$$

We can now integrate equation (5) to obtain the trajectory of the center of mass:

$$(x_{\text{cm}}(t), y_{\text{cm}}(t)) = v_0 \int_0^t (\cos\theta(s), \sin\theta(s)) ds \tag{6}$$

### 1. *Variance for the vertical position:* $\beta \approx 1$

Once we established an analytic solution for the center of mass we can pass to the analysis of the spread of the particles in the $y$ direction and so we want to compute $\sigma_y^2(t) = \langle (y_i(t) - y_{\text{cm}}(t))^2\rangle_i$. In particular using Equation (2)

$$\begin{aligned} y_i(t) &= y_i(0) + \int_0^t \langle \boldsymbol{v}_i(s), \nu_y\rangle \, ds \\ &= y_i(0) + \int_0^t \langle \boldsymbol{v}_{\text{cm}}(s) + (1-\beta) P_{\boldsymbol{v}_{\text{cm}}(t)^\perp}(\boldsymbol{v}_i^{\text{priv}}(s)), \nu_y\rangle \, ds \end{aligned}$$

Now we have to use the particular choice for $\boldsymbol{v}_i^{\text{priv}}$: in the case of *cast and surge* for most of the time the private velocity is in the $y$ direction so $\boldsymbol{v}_i^{\text{priv}} = \nu_y v_i^{\text{priv}}$ and moreover by definition of $\theta$, we have $\langle \boldsymbol{v}_{\text{cm}}(t)^\perp, \nu_y\rangle = \cos(\theta(t))$. So we have

$$\begin{aligned} y_i(t) - y_{\text{cm}}(t) &= \int_0^t \langle \boldsymbol{v}_{\text{cm}}(s), \nu_y\rangle \, ds + \int_0^t \langle (1-\beta) P_{\boldsymbol{v}_{\text{cm}}(t)^\perp}(\boldsymbol{v}_i^{\text{priv}}(s)), \nu_y\rangle \, ds \\ &= y_i(0) - y_{\text{cm}}(0) + (1-\beta) \int_0^t \cos(\theta(s))^2 v_i^{\text{priv}}(s) \, ds. \end{aligned}$$

In order to give an estimate for the last integral we suppose that $\theta$ is moving rather slowly with respect to $v_i^{\text{priv}}$. Letting $c_t = \frac{1}{t}\int_0^t \cos(\theta(s))^2 \, ds$ be the average of $\cos(\theta(s))^2$ in the interval of time considerate we can approximate

$$\int_0^t \cos(\theta(s))^2 v_i^{\text{priv}}(s) \, ds = c_t \int_0^t v_i^{\text{priv}}(s) \, ds = c_t (y_i^{\text{priv}}(t) - y_i^{\text{priv}}(0))$$

Using the fact that $y_i^{\text{priv}}(t) - y_i^{\text{priv}}(0)$ and $y_i(0)$ are independent we obtain

$$\sigma_y^2(t) = \sigma_y^2(0) + (1-\beta)^2 c_t^2 \langle (y_i^{\text{priv}}(t) - y_i^{\text{priv}}(0))^2\rangle_i.$$

Since in our model we have $\boldsymbol{v}_i^{\text{priv}}(t) = (-1)^{a_i} \boldsymbol{v}^{\text{CS}}(t + \gamma_i)$, where $\gamma_i$ is a random timeshift in $[0, t_{clock}]$, and $\boldsymbol{v}^{\text{CS}}$ is the cast and surge program, we can then say

$$\sigma_y^2(t) = \sigma_y^2(0) + \frac{(1-\beta)^2 c_t^2}{t_{clock}} \int_0^{t_{clock}} (y^{\text{CS}}(t+\gamma) - y^{\text{CS}}(\gamma))^2 \, d\gamma \tag{7}$$

In Eq. 7 we note that the swarm spreads little from its initial condition $\sigma_y(0)$, as the second term depends on $(1-\beta)^2$. Importantly, the integral can be calculated explicitly knowing the private velocity, as it does not depend on the kinematics of the center of mass. The constant $c_t$ represents the alignment of the center of mass in the upwind direction ($c_t = 1$ when the center of mass moves upwind, $c_t = 0$ if the center of mass moves crosswind). At low $\beta$, the swarm forgets rapidly its initial condition, and $c_t = 1$ regardless of the initial condition. At large $\beta$, $c_t = 1$ for initial condition (1) only. Note however that because the second term is small owing to the $(1-\beta)^2$ prefactor, we will ignore corrections to $c_t = 1$ at play for other initial conditions.

### B. Very low trust parameter

Remember we are assuming $\boldsymbol{v}_i^{\rm pub}(t) = \boldsymbol{v}^{\rm pub}(t) = v_0 \frac{\boldsymbol{v}_{\rm cm}(t-dt)}{\|\boldsymbol{v}_{\rm cm}(t-dt)\|}$. We now write $\boldsymbol{v}_{\rm cm}(t) = \langle \boldsymbol{v}_i(t)\rangle$ explicitly:

$$\boldsymbol{v}_{\rm cm}(t) = \langle \boldsymbol{v}_i(t)\rangle = \beta v_0 \left\langle \frac{\boldsymbol{v}^{\rm pub}(t)}{\|\beta \boldsymbol{v}^{\rm pub}(t) + (1-\beta)\boldsymbol{v}_i^{\rm priv}(t)\|}\right\rangle + (1-\beta) v_0 \left\langle \frac{\boldsymbol{v}_i^{\rm priv}(t)}{\|\beta \boldsymbol{v}^{\rm pub}(t) + (1-\beta)\boldsymbol{v}_i^{\rm priv}(t)\|}\right\rangle.$$

We use now the peculiar shape of the private velocity. For the *cast and surge*, ignoring the kinks, we have $\boldsymbol{v}_i^{\rm priv}(t) = \pm(0, v_0)$ at each moment. Let us consider $p_+$ the probability of having $\boldsymbol{v}_i^{\rm priv}(t) = (0, v_0)$ and $p_-$ the probability of having $\boldsymbol{v}_i^{\rm priv}(t) = -(0, v_0)$ ($p_+$ and $p_-$ depend on time but for a lighter notation we drop the dependence). Denoting $a_\pm = \frac{v_0}{\|\beta \boldsymbol{v}^{\rm pub}(t) \pm (1-\beta)(0,v_0)\|}$, we get

$$\boldsymbol{v}_{\rm cm}(t) = \beta(a_+p_+ + a_-p_-)\boldsymbol{v}^{\rm pub}(t) + +(1-\beta)(a_+p_+ - a_-p_-)(0, v_0).$$

We use now the more precise assumption on the private velocity $\boldsymbol{v}_i^{\rm priv}(t) = (v_x^{\rm CS}(t+\gamma_i), (-1)^{b_i} v_y^{\rm CS}(t+\gamma_i))$ , where $b_i \in \{-1, +1\}$ and $\gamma_i \in [0, t_{\rm clock}]$ with uniform probability. In particular approximatevely $p_+ = p_- = 1/2$, with a (noise) error of $p_+ - \frac{1}{2} = O(\frac{1}{\sqrt{N}})$, we can thus add and subtract $\frac{1}{2}$ to get

$$\boldsymbol{v}_{\rm cm}(t) = \beta \frac{a_+ + a_-}{2} \boldsymbol{v}^{\rm pub}(t) + (1-\beta)\frac{a_+ - a_-}{2}(0, v_0) + \boldsymbol{\eta}(t),$$

where we keep in mind that the noise $\boldsymbol{\eta}(t) = (1-\beta)\frac{a_+ + a_-}{2} \cdot (2p_+ - 1)\cdot (0, v_0)$ is $O(\frac{v_0}{\sqrt{N}})$. Notice that again thanks to the particular shape of $\boldsymbol{v}_i^{\rm priv}$ we can say write

$$\boldsymbol{\eta}(t) = (1-\beta)\frac{a_+ + a_-}{2}\cdot(2p_+ - 1)\cdot(0, v_0) = (1-\beta)\frac{a_+ + a_-}{2}\cdot \langle \boldsymbol{v}_i^{\rm priv}\rangle; \tag{8}$$

moreover this expression is even more precise since it re-instate the kinks in the computation.
With a Taylor expansion for $a_\pm$ as function of $\beta(1-\beta)$: $a_\pm = 1 - \beta(1-\beta)(-1 \pm v_y^{\rm pub}(t)/v_0) + O(\beta^2(1-\beta)^2)$, we get

$$\boldsymbol{v}_{\rm cm}(t) = \beta \boldsymbol{v}^{\rm pub}(t) - \beta(1-\beta)^2(0, v_y^{\rm pub}(t)) + \boldsymbol{\eta}(t) + O(v_0\beta^2). \tag{9}$$

We can now look at the two regimes:

- $\beta \ll \frac{1}{\sqrt{N}}$. In this case the first two terms are negligible and so as a first approximation $\boldsymbol{v}_{\rm cm}(t) = \boldsymbol{\eta}(t)$
- $\frac{1}{\sqrt{N}} \ll \beta \ll 1$. In this case we have

$$\begin{cases} \boldsymbol{v}^{\rm pub}(t) &= v_0 \frac{\boldsymbol{v}_{\rm cm}(t-t_{\rm mem})}{\|\boldsymbol{v}_{\rm cm}(t-t_{\rm mem})\|} \\ \boldsymbol{v}_{\rm cm}(t) &= \Big(\beta v_x^{\rm pub}(t), (2\beta^2 - \beta^3)v_y^{\rm pub}(t)\Big) + (1-\beta)\cdot \bar{a} \cdot \Big(\langle v_{x,i}^{\rm priv}(t)\rangle, \langle v_{y,i}^{\rm priv}(t)\rangle\Big). \end{cases}$$

Letting $(x_n, y_n) = \frac{\boldsymbol{v}_{\rm cm}(nt_{\rm mem})}{v_0}$ and $(\alpha_n, \beta_n) = (1-\beta)\bar{a}\frac{\langle \boldsymbol{v}_i^{\rm priv}(nt_{\rm mem})\rangle}{v_0}$ we obtain

$$\begin{cases} x_{n+1} &= \beta \frac{x_n}{\sqrt{x_n^2 + y_n^2}} + \alpha_{n+1} \\ y_{n+1} &= (2\beta^2 - \beta^3)\frac{y_n}{\sqrt{x_n^2+y_n^2}} + \beta_{n+1} \end{cases} \xrightarrow{t_n = \frac{y_n}{x_n}} \begin{cases} x_{n+1} &= \beta \frac{1}{\sqrt{1+t_n^2}} + \alpha_{n+1} \\ y_{n+1} &= (2\beta^2 - \beta^3)\frac{t_n}{\sqrt{1+t_n^2}} + \beta_{n+1} \end{cases}$$

$$t_{n+1} = \frac{(2\beta - \beta^2)t_n + \frac{\beta_{n+1}}{\beta}\sqrt{1+t_n^2}}{1 + \frac{\alpha_{n+1}}{\beta}\sqrt{1+t_n^2}} \implies |t_{n+1}| \le \Big(2\beta - \beta^2 + \frac{\beta_{n+1}}{\beta}\Big)|t_n| + \frac{\beta_{n+1}}{\beta}$$

Notice that $\beta_n = O(\frac{1}{\sqrt{N}}) \ll \beta$ while $\alpha_n \sim \frac{1}{\sqrt{t_{\rm clock} + nt_{\rm mem}}}$. Iterating the last inequality we get $|t_n| \le \frac{\beta_n}{\beta}$ exponentially fast and so $x_{n+1} = \beta + \alpha_{n+1} - O(\beta\cdot\beta_n)$ while $y_{n+1} = \beta_{n+1} + O(\beta_n \cdot \beta)$.
In the end, after a small initial regime we converge to

$$\boldsymbol{v}_{\rm cm}(t) = \beta(v_0, 0) + \boldsymbol{\eta}(t) + O(\beta^2),$$

In both regimes, using (8), we can thus approximate

$$\boldsymbol{v}_{\rm cm}(t) = \beta(v_0, 0) + (1-\beta)\cdot\bar{a}\cdot\langle\boldsymbol{v}_i^{\rm priv}\rangle. \tag{10}$$

Integrating out we get

$$(x_{\rm cm}(t), y_{cm}(t)) = (\beta v_0 t + (1-\beta)\bar{a}\langle x_i^{\rm priv}(t)\rangle, (1-\beta)\bar{a}\langle y_i^{\rm priv}(t)\rangle)$$

### 1. *Variance for the vertical position:* $\beta \approx 0$

We need to compute $\sigma_y$, as in the high trust regime. Taylor expanding in $\beta$ we get

$$\boldsymbol{v}_i(t) = \beta\boldsymbol{v}^{\rm pub}(t) + (1-\beta)a_\pm\boldsymbol{v}_i^{\rm priv}(t) = \beta\boldsymbol{v}^{\rm pub}(t) + (1-\beta)\bar{a}\boldsymbol{v}_i^{\rm priv}(t) + o(\beta),$$

where we use that $|\bar{a} - a_\pm| \sim \beta\cdot\frac{v^y_{pub}}{v_0} \ll \beta$ since $\frac{v^y_{cm}}{v^x_{cm}}$ is very small.

Taking the average in $i$ we get

$$\boldsymbol{v}_{\rm cm}(t) = \langle\boldsymbol{v}_i(t)\rangle = \beta\boldsymbol{v}^{\rm pub}(t) + (1-\beta)\bar{a}\langle\boldsymbol{v}_i^{\rm priv}(t)\rangle + o(\beta).$$

Subtracting this from the equation of $\boldsymbol{v}_i(t)$ we get

$$\boldsymbol{v}_i(t) = \boldsymbol{v}_{\rm cm}(t) + (1-\beta)\cdot\bar{a}\cdot\Big(\boldsymbol{v}_i^{\rm priv}(t) - \langle\boldsymbol{v}_i^{\rm priv}(t)\rangle\Big)$$

$$\boldsymbol{v}_i(t) - \boldsymbol{v}_{\rm cm}(t) = \bar{a}\cdot(1-\beta)\cdot\Big(\boldsymbol{v}_i^{\rm priv}(t) - \langle\boldsymbol{v}_i^{\rm priv}(t)\rangle\Big)$$

$$y_i(t) - y_{\rm cm}(t) = y_i(0) + \bar{a}\cdot(1-\beta)\Big(y_i^{\rm priv}(t) - y_i^{\rm priv}(0) - \langle y_i^{\rm priv}(t) - y_i^{\rm priv}(0)\rangle\Big).$$

For our choice of the private velocity we have $y_i^{\rm priv}(t) - y_i^{\rm priv}(0) = (-1)^{\alpha_i}(y^{\rm CS}(t+\gamma_i) - y^{\rm CS}(\gamma_i))$, in particular that the initialization clocks $\gamma_i$ are uniformly taken at random in $[0, t_{\rm clock}]$ and also $\alpha_i \in \{-1, 1\}$ uniformly at random, the average term will be lower order with respect to the first term and so

$$y_i(t) - y_{\rm cm}(t) = y_i(0) + \bar{a}\cdot(1-\beta)\cdot(-1)^{\alpha_i}(y^{\rm CS}(t+\gamma_i) - y^{\rm CS}(\gamma_i))$$

By the independence of the initialization $y_i(0)$ and the private velocity we obtain

$$\sigma_y^2(t) = \langle(y_i(t) - y_{\rm cm}(t))^2\rangle = \langle y_i(0)^2\rangle + \bar{a}^2\cdot(1-\beta)^2\cdot\langle\big(y^{\rm CS}(t+\gamma_i) - y^{\rm CS}(\gamma_i)\big)^2\rangle_i;$$

Using finally that $\gamma_i \in [0, t_{\rm clock}]$ uniformly we get

$$\sigma_y^2(t) = \sigma_y^2(0) + [1 + (2\beta(1-\beta))]\frac{(1-\beta)^2}{t_{\rm clock}}\cdot\int_0^{t_{\rm clock}}(y^{\rm CS}(t+\gamma) - y^{\rm CS}(\gamma))^2\,d\gamma \tag{11}$$

### C. General noise

Remember we are assuming $\boldsymbol{v}_i^{\text{pub}}(t) = \boldsymbol{v}^{\text{pub}}(t) = v_0 \frac{\boldsymbol{v}_{\text{cm}}(t-dt)}{\|\boldsymbol{v}_{\text{cm}}(t-dt)\|}$. We now write $\boldsymbol{v}_{\text{cm}}(t) = \langle \boldsymbol{v}_i(t) \rangle$ explicitely:

$$\boldsymbol{v}_{\text{cm}}(t) = \langle \boldsymbol{v}_i(t) \rangle = \beta v_0 \left\langle \frac{\boldsymbol{v}^{\text{pub}}(t)}{\|\beta \boldsymbol{v}^{\text{pub}}(t) + (1-\beta)\boldsymbol{v}_i^{\text{priv}}(t)\|} \right\rangle + (1-\beta) v_0 \left\langle \frac{\boldsymbol{v}_i^{\text{priv}}(t)}{\|\beta \boldsymbol{v}^{\text{pub}}(t) + (1-\beta)\boldsymbol{v}_i^{\text{priv}}(t)\|} \right\rangle .$$

We use now the peculiar shape of the private velocity. Let $a_i(t) = \frac{v_0}{\|\beta \boldsymbol{v}^{\text{pub}}(t) \pm (1-\beta)\boldsymbol{v}_i^{\text{priv}}(t)\|}$ and let us do a Taylor expansion for $a_i$ as function of $\beta(1-\beta)$:

$$\begin{aligned} a_i(t) &= \frac{v_0}{\|\beta \boldsymbol{v}^{\text{pub}}(t) \pm (1-\beta)\boldsymbol{v}_i^{\text{priv}}(t)\|} = \frac{v_0}{\sqrt{\beta^2 v_0^2 + (1-\beta)^2 v_0^2 + 2\beta(1-\beta)\langle \boldsymbol{v}^{\text{pub}}(t), \boldsymbol{v}_i^{\text{priv}}(t)\rangle}} \\ &= \frac{1}{\sqrt{\beta^2 + (1-\beta)^2 + 2\beta(1-\beta)\frac{\langle \boldsymbol{v}^{\text{pub}}(t), \boldsymbol{v}_i^{\text{priv}}(t)\rangle}{v_0^2}}} = \left(1 + 2\beta(1-\beta)\Big(-1 + \frac{\langle \boldsymbol{v}^{\text{pub}}(t), \boldsymbol{v}_i^{\text{priv}}(t)\rangle}{v_0^2}\Big)\right)^{-\frac{1}{2}} \\ &= 1 - \beta(1-\beta)\Big(-1 + \frac{\langle \boldsymbol{v}^{\text{pub}}(t), \boldsymbol{v}_i^{\text{priv}}(t)\rangle}{v_0^2}\Big) + O(\beta^2(1-\beta)^2). \end{aligned}$$

Let us now denote $\boldsymbol{\eta}(t) = \langle \boldsymbol{v}_i^{\text{priv}}(t) \rangle$ the expectation of the private velocity and $Q(t) = \frac{1}{v_0^2}\langle \boldsymbol{v}_i^{\text{priv}}(t) \otimes \boldsymbol{v}_i^{\text{priv}}(t) \rangle$ the renormalized covariance operator of the private velocity. Notice that we always have $Q(t) \succeq 0$ and $\text{tr}(Q) = 1$. For the cast and surge case we have an even more explicit structure

$$Q(t) \approx \begin{pmatrix} \alpha(t) & 0 \\ 0 & 1-\alpha(t) \end{pmatrix} \qquad \text{where } \alpha(t) = \frac{1}{\sqrt{2}v_0}\eta_x(t).$$

Now

$$\begin{aligned} \boldsymbol{v}^{\text{pub}}(t)\langle a_i \rangle &= (1 + \beta(1-\beta))\boldsymbol{v}^{\text{pub}}(t) - \beta(1-\beta)\boldsymbol{v}^{\text{pub}}(t)\frac{\langle \boldsymbol{v}^{\text{pub}}(t), \boldsymbol{\eta}(t)\rangle}{v_0^2} \\ &= (1 + \beta(1-\beta))\boldsymbol{v}^{\text{pub}}(t) - \beta(1-\beta)P_{\boldsymbol{v}^{\text{pub}}(t)}(\boldsymbol{\eta}(t)) \end{aligned}$$

$$\langle \boldsymbol{v}_i^{\text{priv}}(t) a_i \rangle = (1 + \beta(1-\beta))\boldsymbol{\eta}(t) - \beta(1-\beta)Q(t)\boldsymbol{v}^{\text{pub}}(t).$$

Finally we get

$$\begin{aligned} \boldsymbol{v}_{\text{cm}}(t) &= \beta \boldsymbol{v}^{\text{pub}}(t)\langle a_i \rangle + (1-\beta)\langle a_i \boldsymbol{v}_i^{\text{priv}}(t) \rangle \\ &= \Big(\beta + \beta^2(1-\beta) - \beta(1-\beta)^2 Q(t)\Big)\boldsymbol{v}^{\text{pub}}(t) + \Big((1-\beta) + \beta(1-\beta)^2 - \beta^2(1-\beta)P_{\boldsymbol{v}^{\text{pub}}(t)}\Big)\boldsymbol{\eta}(t) \end{aligned}$$

In the different regimes $\beta \approx 1$ and $\beta \approx 0$, we can then arrive to the more concise forms:

$$\begin{aligned} \boldsymbol{v}_{\text{cm}}(t) &= \boldsymbol{v}^{\text{pub}}(t) + (1-\beta)\big(1 - P_{\boldsymbol{v}^{\text{pub}}(t)}\big)\boldsymbol{\eta}(t) + O((1-\beta)^2) \\ \boldsymbol{v}_{\text{cm}}(t) &= \beta\big(1 - Q(t)\big)\boldsymbol{v}^{\text{pub}}(t) + \boldsymbol{\eta}(t) + O(\beta^2) \end{aligned}$$

### D. Pair of synchronous agents

The timescale for a pair of synchronous agents to perform their sharp turn depends on both $\beta$ and $t_{\text{mem}}$. To quantify this timescale, let us define the angle $\theta_t^i$ the agents velocity, $\boldsymbol{v}_i(t)$, makes with the horizontal: $\boldsymbol{v}_i(t) = v_0(\cos(\theta_t^i), \sin(\theta_t^i))$. Given that we have $N = 2$, in this case it is obvious that $\boldsymbol{v}_i^{\text{priv}}(t) = \boldsymbol{v}_j(t - t_{\text{mem}})$, but the behavior of each particle will

be the same if they are synchronous, so in the end $\boldsymbol{v}_i^{\text{priv}}(t) = \boldsymbol{v}_i(t - t_{\text{mem}})$. When $\boldsymbol{v}_i^{\text{priv}} = \hat{y}$ from eq. (1) in the main paper, we then have that

$$v_0(\cos(\theta_t^i), \sin(\theta_t^i)) = v_0 \frac{(\beta\cos(\theta^i_{t-t_{\text{mem}}}), \beta\sin(\theta^i_{t-t_{\text{mem}}}) + (1-\beta))}{(\beta\cos(\theta^i_{t-t_{\text{mem}}}), \beta\sin(\theta^i_{t-t_{\text{mem}}}) + (1-\beta))\|};$$

in particular we deduce

$$\tan(\theta_t^i) = \frac{\sin(\theta_t^i)}{\cos(\theta_t^i)} = \frac{\sin(\theta^i_{t-t_{\text{mem}}}) + (1-\beta)}{\beta\cos(\theta^i_{t-t_{\text{mem}}})} = \tan(\theta^i_{t-t_{\text{mem}}}) + \frac{1-\beta}{\beta\cos(\theta^i_{t-t_{\text{mem}}})}.$$

We assume now $t_{\text{mem}} \ll 1$ so that

$$\frac{1-\beta}{\beta\cos(\theta^i_{t-t_{\text{mem}}})} = \tan(\theta_t^i) - \tan(\theta^i_{t-t_{\text{mem}}}) \approx t_{\text{mem}} \cdot \dot{\theta}^i_{t-t_{\text{mem}}} \cdot \frac{1}{\cos(\theta^i_{t-t_{\text{mem}}})^2},$$

which let us consider $\dot{\theta}_t^i \approx \frac{1-\beta}{\beta t_{\text{mem}}} \cos(\theta_t^i)$ . Let $\tau = \frac{t_{\text{mem}}}{1-\beta}$; the solution of the ODE is $\frac{1+\sin(\theta_t^i)}{\cos(\theta_t^i)} = Ae^{\frac{t}{\tau}}$ hence the time to switch from $\theta^i_{t_-} = -\frac{\pi}{2} + \varepsilon$ to $\theta^i_{t_+} = \frac{\pi}{2} - \varepsilon$ is $\Delta t \approx 2\tau|\log(\varepsilon/2)|$, in fact

$$Ae^{\frac{t_+}{\tau}} = \frac{1+\sin(\theta^i_{t_+})}{\cos(\theta^i_{t_+})} \approx \frac{2}{\varepsilon} \qquad Ae^{\frac{t_-}{\tau}} = \frac{1+\sin(\theta^i_{t_-})}{\cos(\theta^i_{t_-})} = \frac{\cos(\theta^i_{t_-})}{1-\sin(\theta^i_{t_-})} \approx \frac{\varepsilon}{2}$$

and so $e^{\frac{\Delta t}{\tau}} = e^{\frac{t_+ - t_-}{\tau}} \approx \frac{4}{\varepsilon^2}$ from which $\Delta t \approx 2\tau|\ln(\varepsilon/2)| = \frac{t_{\text{mem}}}{1-\beta} \cdot 2\beta|\log(\varepsilon/2)|$.

## III. SUPPLEMENTARY FIGURES

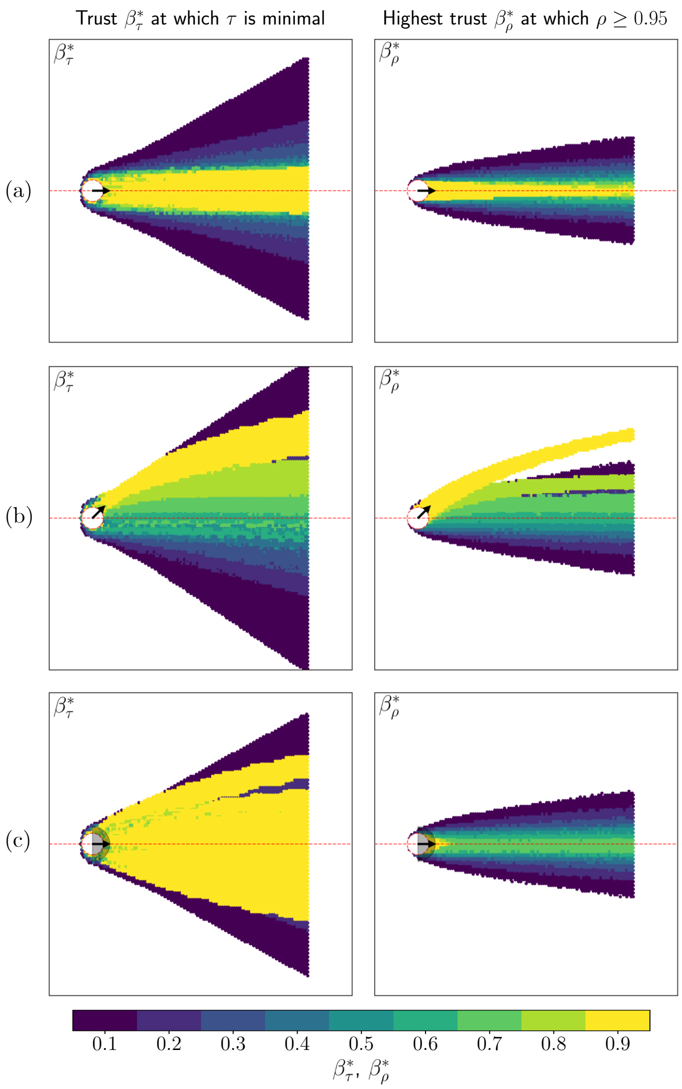


FIG. 1. Maps showing the optimal values $\beta_\tau^*$, $\beta_\rho^*$ at which points in space are reached respectively with minimal first-passage time $\tau$ (left column) and success rate $\rho \geq 0.95$ (right column). Rows correspond to different initial conditions: (a) $\mu = 0$, $\sigma = 0$; (b) $\mu = \pi/4$, $\sigma = 0$; (c) $\mu = 0$, $\sigma = \pi/2$.
